# Supplementary material for: Unveiling the growth mode diagram of GaSe on sapphire
Source: arXiv:2510.10743 ancillary file (2025-10-12)
Supplement: Supplementary file 1 [file Supplementary_Information.pdf]

# Supplementary Information

## Unveiling the growth mode diagram of GaSe on sapphire

*M. Bissolo[1] ⁎, M. Dembecki[1], J. Belz[2], J. Schabesberger[1], M. Bergmann[2], P. Avdienko[1], F. Rauscher[1], A. S. Ulhe[1], H. Riedl[1], K. Volz[2], J. J. Finley,[1] E. Zallo[1]†, and G. Koblmüller[1,3]*

*1)Walter-Schottky-Institut and TUM School of Natural Sciences, Technische Universität München, Am Coulombwall 4, 85748 Garching, Germany*

*2)mar.quest | Marburg Center for Quantum Materials and Sustainable Technologies and Department of Physics, Philipps-Universität Marburg, 35032 Marburg, Germany*

*3)Institute of Solid State Physics, Technical University Berlin, 10623 Berlin, Germany*

**E-mail:* michele.bissolo@tum.de

*†E-mail:* eugenio.zallo@tum.de

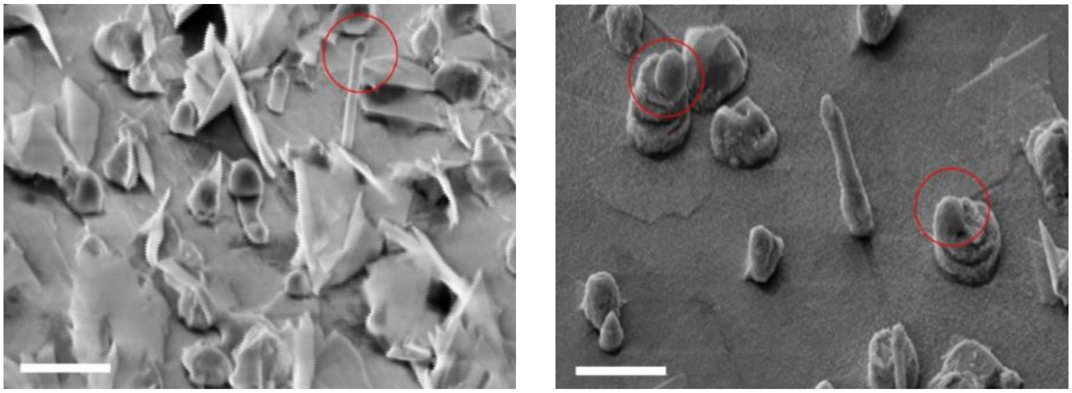

**Figure S 1:** SEM images of different structures displaying a droplet (red circle) on the top, indicating a VLS-type growth. Scalebar: 2 µm.

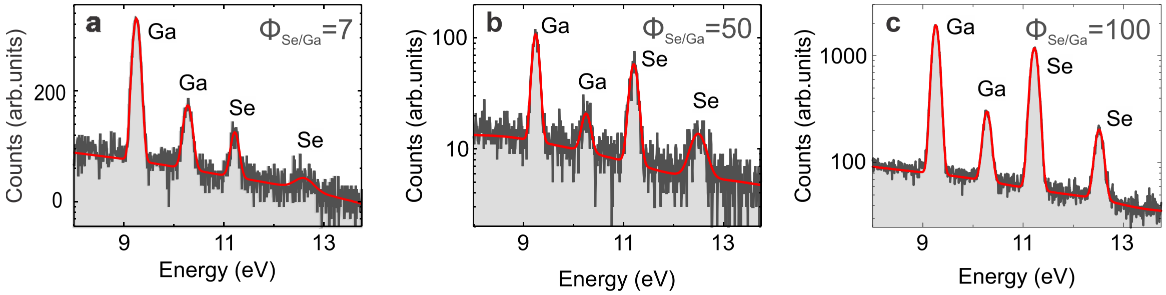


**Figure S 2:** (a-c) EDX spectra of clusters formed at Se/Ga flux ratios of 7, 50 and 100, respectively. The red lines are Gaussian fits of the peaks. At low flux ratios, the clusters predominantly consist of gallium, while at higher flux ratios the Se content increases.

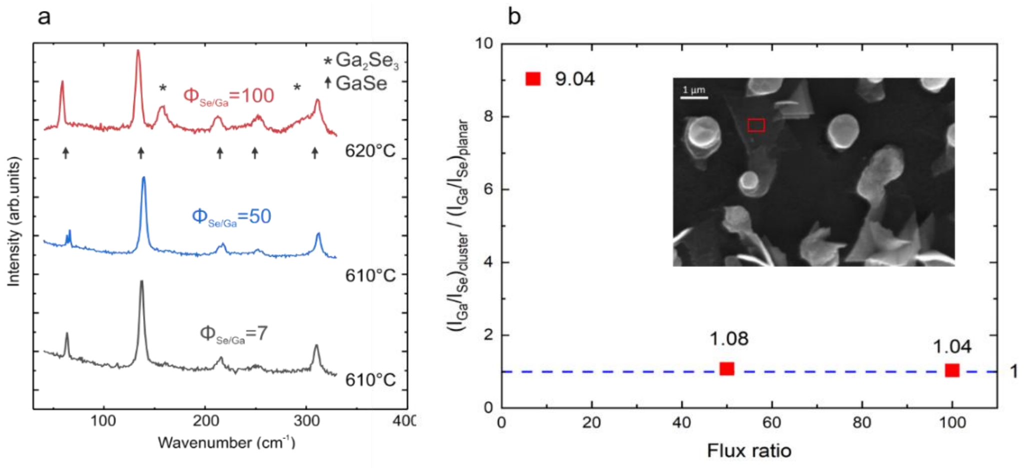


**Figure S 3:** (a) Raman spectra from clusters at different Se/Ga flux ratios and substrate temperatures. At the highest measured flux ratios the clusters consist of both the 2:3 and 1:1 phase, due to the higher relative Se flux. (b) EDX area ratio (Ga/Se) of clusters divided by the EDX area ratio of triangular GaSe measured between the clusters (see highlighted area in the inset).

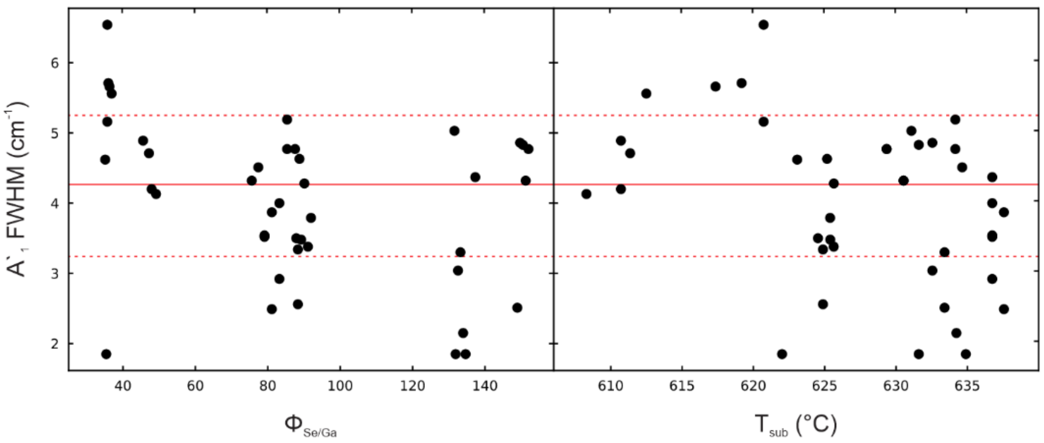


**Figure S 4:** FWHM of the A’$_1$ Raman mode of GaSe extracted from various growths and plotted as a function of substrate temperature ($T_{sub}$) and flux ratio ($\Phi_{Se/Ga}$). The continuous red line indicates the mean value out of 5 FWHM measurements of exfoliated GaSe (measured in the same setup), while the dotted red line indicates the largest and smallest values.

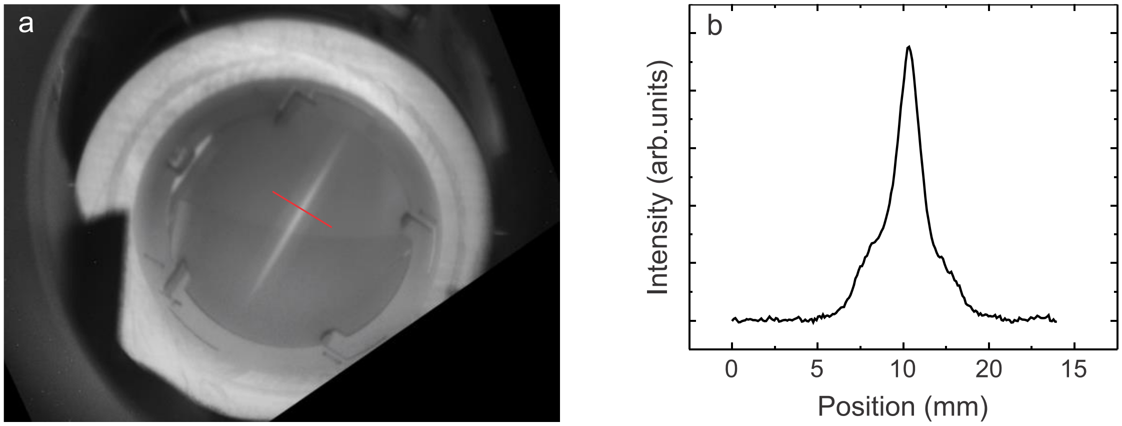


**Figure S 5: (**a) RHEED cathodoluminescence of sapphire showing that the probed area covers most of the wafer. The RHEED parameters were chosen to optimize the focus on the RHEED screen. The red linecut perpendicular to the RHEED beam direction is shown in (b).

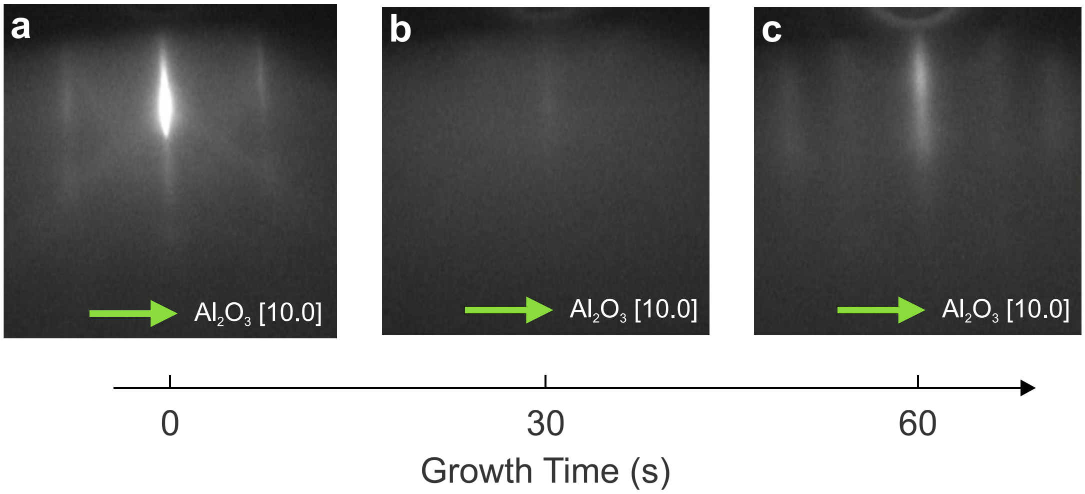


**Figure S 6:** Darkening of the substrate pattern in the first stages of growth. (a) Sapphire pattern before the growth, (b) RHEED pattern after 30 seconds of growth showing features typical of amorphous films, and (c) RHEED pattern after 1 minute of growth with the characteristic streaks of the $Ga_2Se_2$ growth.

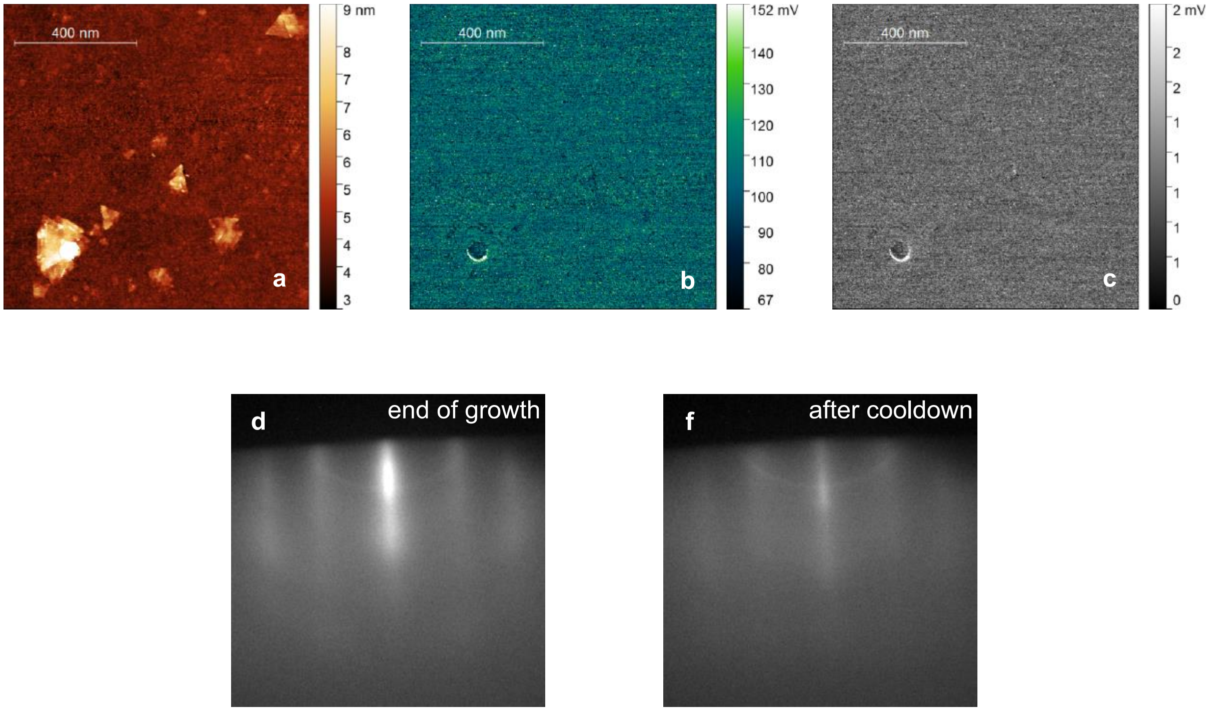


**Figure S 7** (a) Topography of GaSe grown at 625°C and a flux ratio of 30 (desorption regime in Figure 4), showing small isolated flakes. (b) Indentation and (c) adhesion maps of (a) show no contrast between the GaSe flakes and the substrate. (d-e) RHEED patterns from the sample shown in (a-c) right at the end of the growth and after cooldown. The thermal degradation leads to a drastic reduction in the intensity. The diffraction streaks of the sapphire substrate cannot be discerned, indicating that the surface is still covered by a thin GaSe layer with low crystallinity.

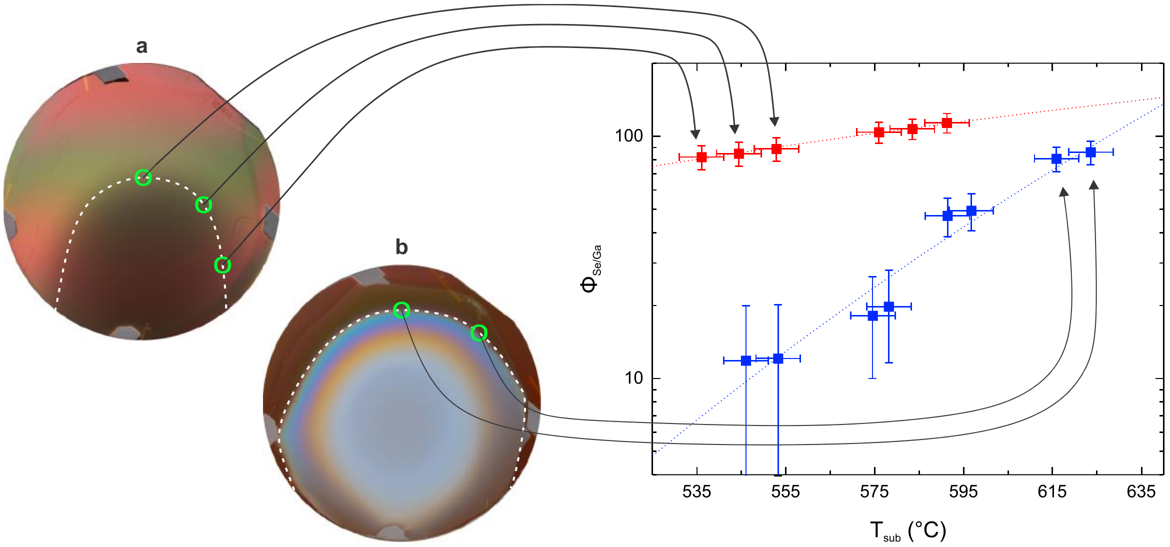


**Figure S 8:** Selected positions in phase space of the morphological transitions are mapped from wafer coordinates (see Figure S3 for more details) onto the phase diagram in cartesian coordinates. The mapping procedure is shown here for (a) a $Ga_2Se_3$ (top) to 3D-nanoflakes (bottom) transitions, and (b) a 3D-nanoflakes (top) to clusters (bottom) transition.

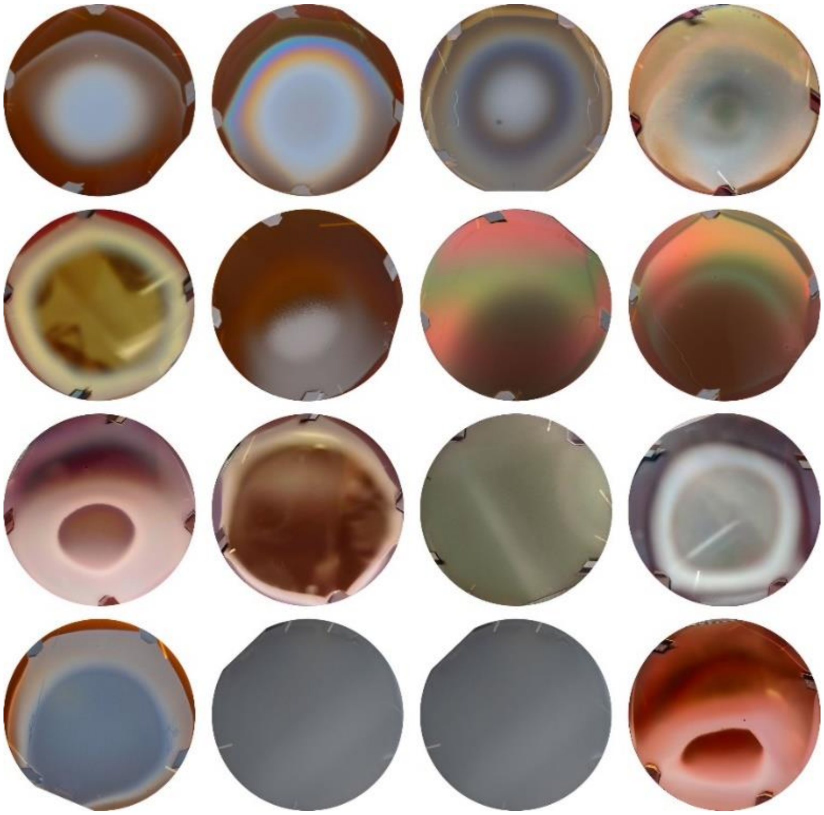

**Figure S 9:** Selected photographs of the GaSe-deposited sapphire wafers.

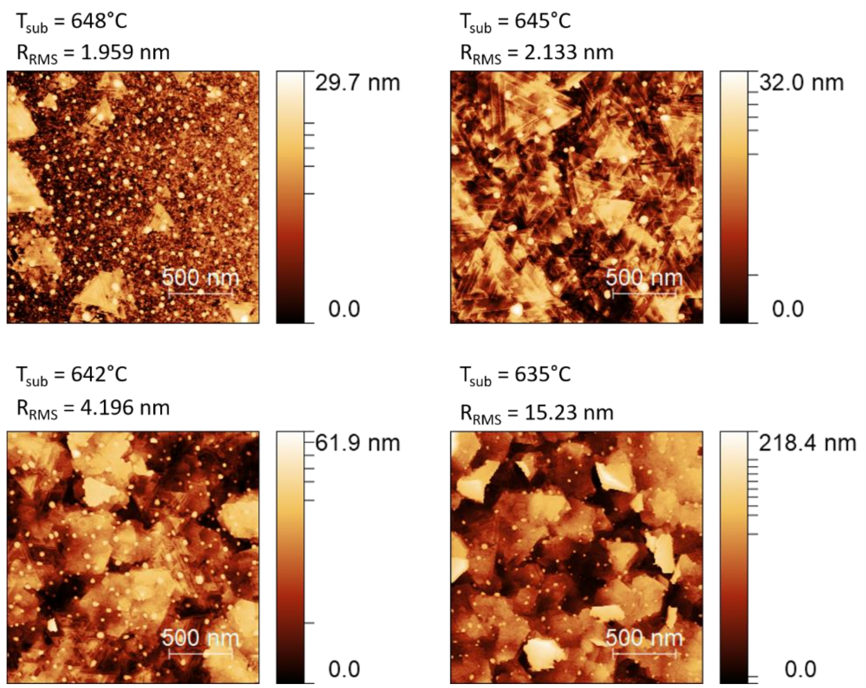


**Figure S 10:** AFM maps of the GaSe growth on sapphire at a Se/Ga flux ratio of 87 as a function of substrate temperature.

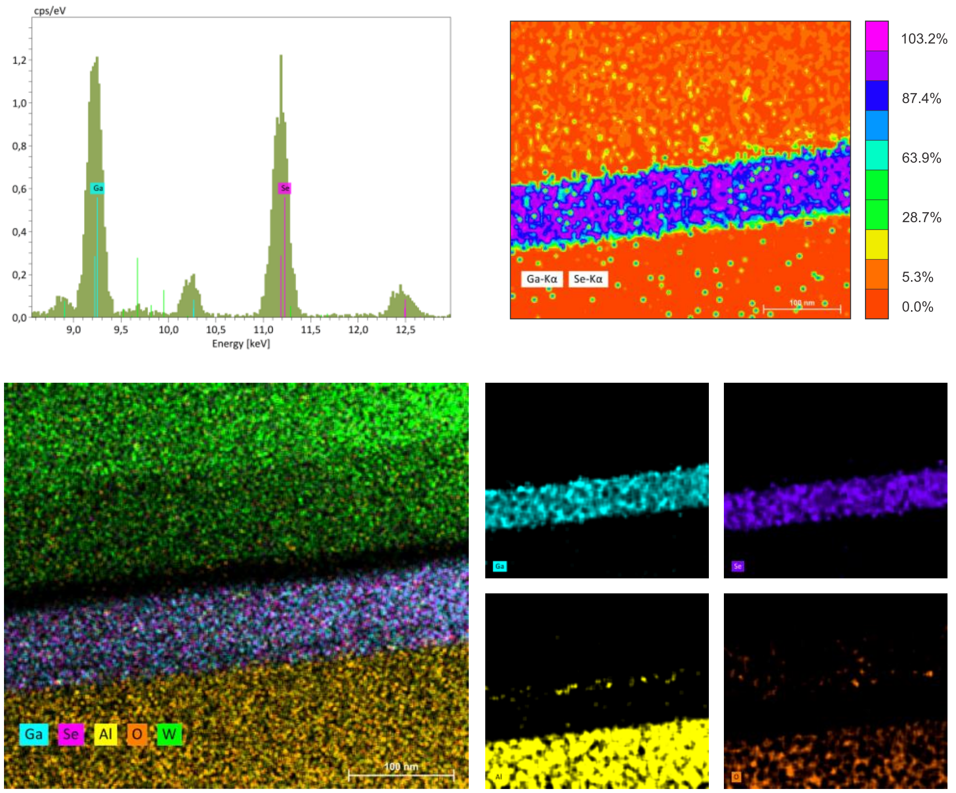


**Figure S 11:** STEM-EDXS showing the 1:1 stoichiometry of the GaSe film.

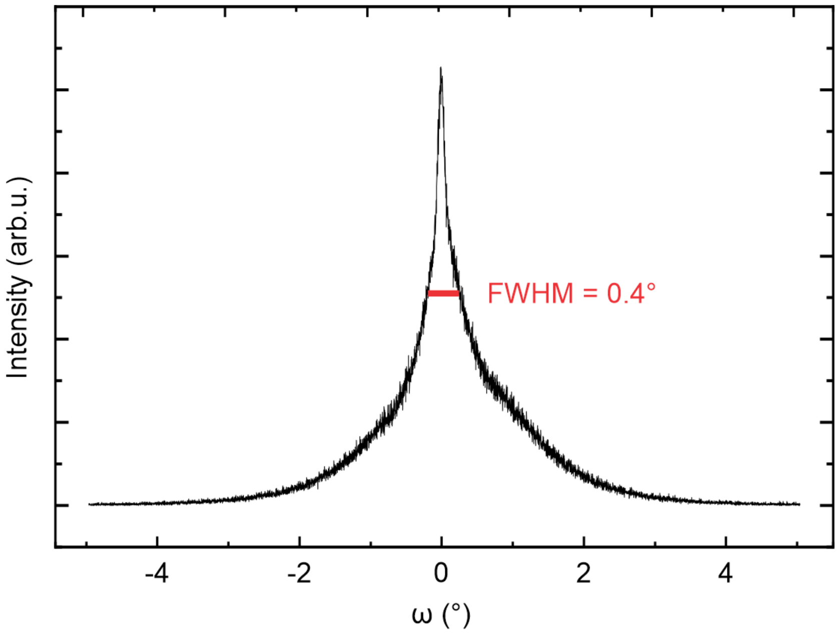


**Figure S 12:** Rocking curve of GaSe around the (006) plane.

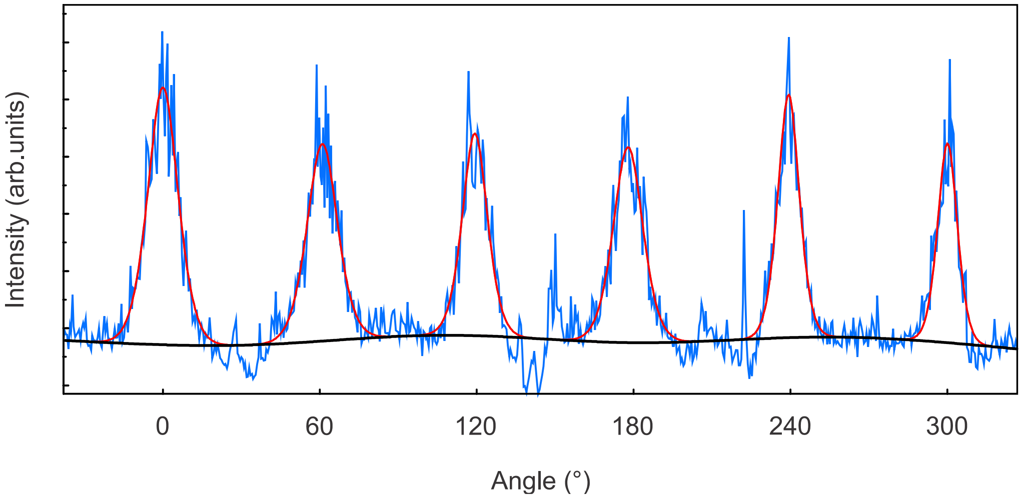


**Figure S 13:** Azimuthal linecut along the dashed green line in the RHEED pole figure in Figure 5 (main text) showing a six-fold periodicity indicative of a hexagonal lattice. The peaks are fitted with a Gaussian/Lorentzian product formula with a mixing of 50. The background is approximated with a linear spline. The peaks (solid red lines) account for 51% of the total area, while the background (solid black line) to 49%.

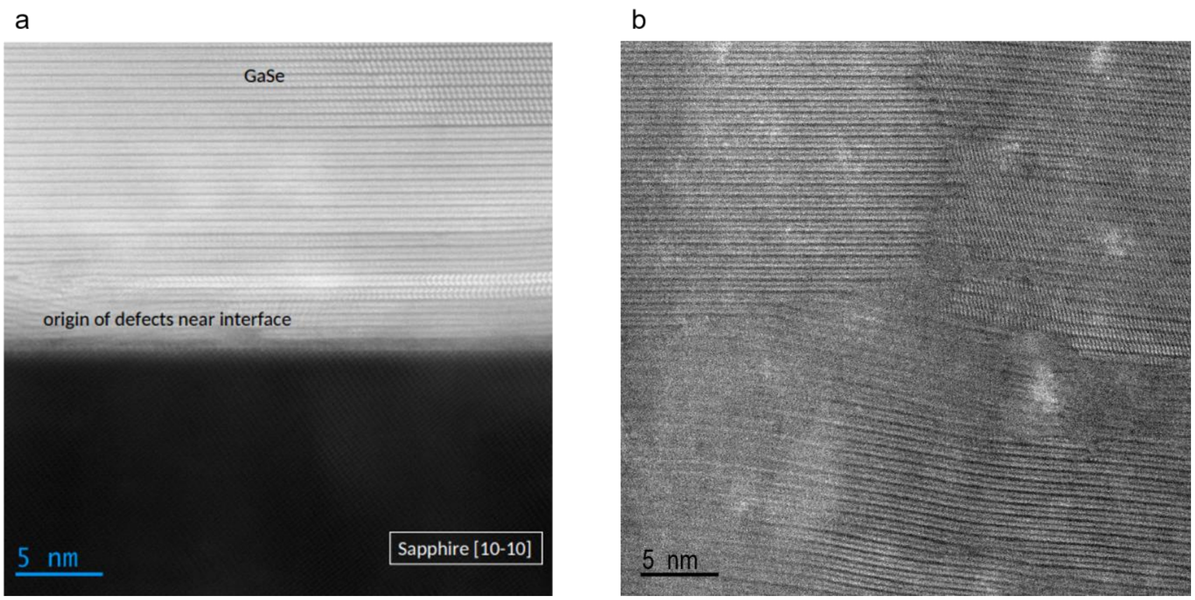


**Figure S 14:** (a) Cross-sectional STEM image of the GaSe/Sapphire interface showing defects and the insertion of defect planes at the interface. In-plane disorder, with various GaSe layers rotated relative to each other, is also visible. (b) Cross-sectional STEM image of an 87 nm-thick GaSe layer on sapphire showing that the film growth occurs through the confluence of grains.

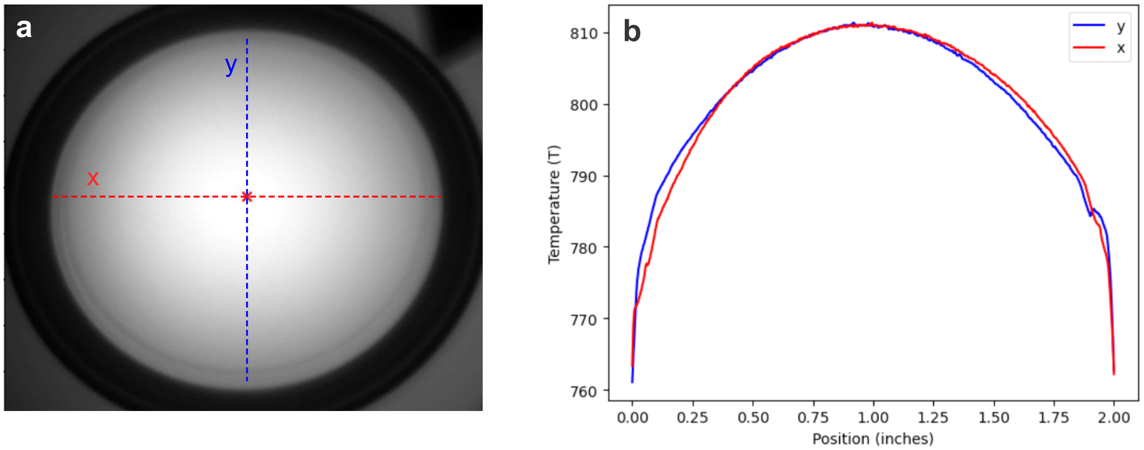


**Figure S 15: (**a) Imaging of the infrared emission of a silicon substrate averaged over a rotation. (b) Temperature profile extracted from the linecuts in (a). The temperature distribution is measured at various heating powers and interpolated between them.

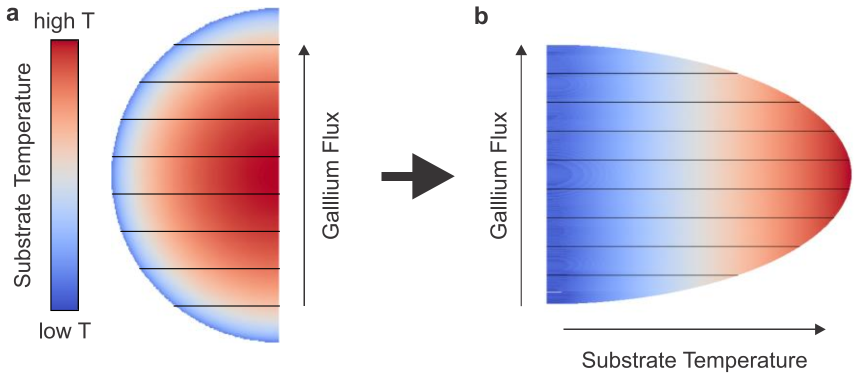


**Figure S 16:** (a) Simulated distribution of substrate temperature and Ga flux across half of the 2-inch wafer. The temperature distribution only depends on the radius, while the Ga flux increases linearly across the wafer. The panel (b) represents a projection to cartesian coordinates, where the x- and y-axes correspond to temperature and gallium flux, respectively. After deposition, the growth on the 2-inch wafer effectively provides a snapshot of a specific region of phase space.

**Note S1: Model for the extrapolation of the ratio of the Raman modes in Figure 3a :**

The ratio of the Raman modes (R) in Figure 3a (main text) is expressed as the product of two functions $f(\Phi_{Se/Ga}) \cdot g(T)$. For $g(T)$ we assume an Arrhenius-type behavior with $g(\mathrm{T}) = A * e^{E/kT}$, where $E$ is the energy scale for the system (which is the combination of various dynamical effects, such as sticking coefficient, desorption rate, etc), $k$ is the Boltzmann constant, $A$ a scaling factor, and $T$ the temperature. The dependence on the flux ratio $f(\Phi_{Se/Ga})$ is highly complex and influenced by various factors such as sticking coefficients, surface kinetics, and material-specific interactions. We thus adopt an empirical exponential function, $f(\Phi_{Se/Ga}) = B * e^{\alpha \cdot \Phi_{\frac{Se}{Ga}} + \beta}$, where $B$, $\alpha$ and $\beta$ are fitting parameters. Thus, the final expression for the extrapolating function is $R = C * e^{\frac{E}{kT} + \alpha \cdot \Phi_{\frac{Se}{Ga}} + \beta}$, where $C$ is $A \cdot B$.
